# Supplementary material for: Nested Weighted Limit-Average Automata of Bounded Width
Source: arXiv:1606.03598 source file (2016-06-11)
Supplement: Supplementary file 1 [file appendix-AMC.tex]

\section{Automata with Monitor Counters}\label{sec:appmc}
\newcommand{\autDiff}{\aut_{\textrm{diff}}}

Automata with monitor counter have been introduced in~\cite{ChatterjeeHO15}, 
and their equivalence with NWA with bounded width has also been 
established in~\cite{ChatterjeeHO15}. 
For the sake of completeness, we present the proof of the equivalence.
However, note that none of the result of this paper depends on this 
equivalence.
We start with an intuitive description of automata with monitor counters.

Automata with monitor counters are intuitively extension of weighted automata
with counters, where the transitions do not depend on the counter value.
We define them formally below.
\smallskip

\Paragraph{Automata with monitor counters.} 
\newcommand{\counterA}{{\cal A}^{\textrm{m-c}}}
An \emph{automaton with $n$ monitor counters} $\counterA$ is a tuple $\tuple{ \Sigma, Q, Q_0, \delta, F}$  where 
(1)~$\Sigma$ is the alphabet,
(2)~$Q$ is a finite set of states,
(3)~$Q_0 \subseteq Q_0$ is the set of initial states,
(4)~$\delta$ is a finite subset of  $Q \times \Sigma \times Q \times (\Z \cup \{ s,t \})^n$ called a transition relation, 
%(the component $(\Z \cup \{ s,t \})^n$ contains an $n$-element sequence of instruction for $n$ monitor counters such as
(each component refers to one monitor counter, where letters $s,t$ refer to starting  and terminating the  counter, 
respectively, and the value from $\Z$ is the value that is added to the counter), and
(5)~$F$ is the set of accepting states. 
Moreover, we assume that for every $(q,a,q',\vec{u}) \in \delta$, at most one component in $\vec{u}$ contains $s$, i.e.,
at most one counter is activated at each position.
Intuitively, the automaton $\counterA$ is equipped with $n$ counters. 
The transitions of $\counterA$ do not depend on the values of counters (hence, we call them monitor counters); and
every transition is of the form $(q,a,q',\vec{v})$, which means that
if $\counterA$ is in the state $q$ and the current letter is $a$, then
it can move to the state $q'$ and update counters according to $v$.
Each counter is initially inactive. It is activated by the instruction $s$, and 
it changes its value at every step by adding the value between $-N$ and $N$
until termination $t$.
The value of the counter at the time it is terminated is then assigned to the position where it has been activated.
An automaton with monitor counters $\counterA$ is \emph{deterministic} if and only if $Q_0$ is a singleton and $\delta$ is a function
from $Q \times \Sigma$ into $Q \times (\Z \cup \{ s,t \})^n$.
\smallskip

\Paragraph{Semantics of automata with monitor counters.} 
A sequence $\run$ of elements from $Q \times (\Z \times \{\bot\})^n$ is a \emph{run} of $\counterA$ on a word $w$
if  (1)~$\run[0] = \tuple{q_0, \vec{\bot}}$ and $q_0 \in Q_0$
and (2)~for every $i > 0$, if $\run[i-1] = \tuple{q,\vec{u}}$
and $\run[i] = \tuple{q', \vec{u}'}$ then $\counterA$ has a transition 
$(q,w[i],q',\vec{v})$ and for every $j \in [1,n]$ we have
(a)~if $v[j] = a$, then $u[j] = \bot$ and $u'[j] = 0$,  
(b)~if $v[j] = t$, then $u[j] \in \Z$ and $u'[j] = \bot$, and
(c)~if $v[j] \in \Z$, then $u'[j] = u[j] + v[j]$.
A run $\run$ is \emph{accepting} if some state from $F$ occurs infinitely often on the first component of $\run$,
infinitely often some counter is activated and every activated counter is finally terminated.
An accepting run $\run$ defines a sequence $\weightedRun$ 
of integers and $\bot$ as follows: let the counter started at position $i$ be $j$, and 
let the value of the counter $j$ terminated at the earliest position after $i$ be $x_j$,
then $\weightedRun[i]$ is $x_j$.
The semantics of automata with monitor counters is given, similarly to weighted automata,
by applying the value function to $\weightedRun$.

\begin{remark}
Automata with monitor counters are very similar in spirit to the register automata considered 
in the works of~\cite{DBLP:conf/lics/AlurDDRY13}. The key difference is that we consider infinite words and value functions 
associated with them, whereas previous works consider finite words.
Another key difference is that in this work we will consider probabilistic semantics, and 
such semantics has not be considered for register automata before.
\end{remark}

We now present translations from NWA to automata with monitor counters and vice-versa.

\begin{restatable}{lemma}{MCvsNested}[Translation Lemma]
\label{l:mc-vs-nested}
For every value function $f \in \InfVal$ on infinite words we have the following:
(1)~Every deterministic $f$-automaton with monitor counters $\counterA$ can be transformed in polynomial time 
into an equivalent deterministic $(f;\fsum)$-automaton of bounded width. %( and polynomial size in $|\counterA|$.)
(2)~Every non-deterministic (resp., deterministic) $(f;\fsum)$-automaton of bounded width can be transformed in exponential time
into an equivalent non-deterministic (resp., deterministic) $f$-automaton with monitor counters.
\end{restatable}
\begin{proof}
%First, we show that deterministic $(f;\fsum)$-automata of bounded width subsume 
%deterministic $f$-automata with monitor-counters. 
\Paragraph{(Translation of automata with monitor counters to NWA)}: Consider a deterministic $f$-automaton $\counterA$ with $k$ monitor counters.
We define an $(f;\fsum)$-automaton $\nestedA$, which consists of a master automaton $\masterA$ and
slave automata $\slaveA_1, \ldots, \slaveA_{k+1}$ defined as follows.
The slave automaton $\slaveA_{k+1}$ is a dummy automaton, i.e., it has only a single state which is both 
the initial and the accepting state. Invoking such an automaton is equivalent to taking a silent transition (with no weight).
Next, the master automaton $\masterA$ and slave automata $\slaveA_1, \ldots, \slaveA_k$ are variants of $\counterA$, i.e., they share the underlying transition structure.
The automaton $\masterA$ simulates $\counterA$, i.e., it has the same states and the transitions among these states as $\counterA$.
However, whenever $\counterA$ activates counter $i$, the master automaton invokes the slave automaton $\slaveA_i$. The accepting condition of $\masterA$ is the same as of $\counterA$.
Slave automata $\slaveA_1,\ldots, \slaveA_k$ keep track of counters $1, \ldots, k$, i.e., 
for every $i \in \{1,\ldots, k\}$, the slave automaton $\slaveA_i$ simulates $\counterA$ and applies instructions of $\counterA$ for counter $i$
to its value. That is, whenever $\counterA$ changes the value of counter $i$ by $m$, the automaton $\slaveA_i$ 
takes a transition of the weight $m$. Finally, $\slaveA_i$ terminates precisely when $\counterA$ terminates counter $i$.
The semantics of automata with monitor counters implies that $\nestedA$ accepts if and only if $\counterA$ accepts and, for every word,
the sequences of weights produced by the runs of $\nestedA$ and $\counterA$ on that word coincide. Therefore, 
the values of $\nestedA$ and $\counterA$ coincide on every word.

\Paragraph{(Translation of NWA of bounded width to automata with monitor counters)}: We show that non-deterministic (resp., deterministic) 
$f$-automata with monitor counters  subsume 
non-deterministic (resp., deterministic) $(f;\fsum)$-automata of bounded width. 
Consider a non-deterministic $(f;\fsum)$-automaton $\nestedA$ with width bounded by $k$. 
We define an $f$-automaton $\counterA$ with $k$ monitor counters that works as follows. 
Let $Q_{mas}$ be the set of states of the master automaton of $\nestedA$ and $Q_s$ be the union of the sets of states of the slave automata of $\nestedA$.
The set of states of $\counterA$ is $Q_{mas} \times Q_{s} \times \ldots \times Q_s =
Q_{mas} \times (Q_s)^k$. 
The automaton $\counterA$ simulates runs of the master automaton and slave automata by keeping track of the state of the master automaton and 
states of up to $k$ active slave automata. 
Moreover, it uses counters to simulate the values of slave automata, i.e., 
whenever a slave automaton is activated, $\counterA$ simulates the execution of this automaton and
assigns some counter $i$ to that automaton. 
Next, when the simulated slave automaton takes a transition of the weight $m$ the automaton $\counterA$
changes the value of counter $i$ by $m$.
Finally, $\counterA$ terminates counter $i$ when the corresponding slave automaton terminates.

Since $\nestedA$ has width bounded by $k$, the simulating automaton $\counterA$ never runs out of counters to simulate slave automata. 
Moreover, as it simulates runs of the master automaton and slave automata of $\nestedA$, there is a one-to-one
correspondence between runs of $\counterA$ and runs of $\nestedA$ and accepting runs of $\nestedA$ correspond to accepting runs of $\counterA$.
Finally, the sequence of weights for the master automaton determined by a given run of $\nestedA$ coincides with the sequence of 
weights of $\counterA$ on the corresponding run. Therefore, the values of $\nestedA$ and $\counterA$ coincide on every word.
Thus, non-deterministic $f$-automata with monitor counters  subsume 
non-deterministic $(f;\fsum)$-automata of bounded width. Moreover, 
the one-to-one correspondence between runs of $\nestedA$ and $\counterA$ implies that if $\nestedA$ is deterministic, then $\counterA$ is deterministic. 
Therefore, deterministic $f$-automata with monitor counters  subsume 
deterministic $(f;\fsum)$-automata of bounded width. This completes the proof.
\end{proof}
